# Supplementary material for: Beyond Alignment: Blind Video Face Restoration via Parsing-Guided Temporal-Coherent Transformer
Source: arXiv:2404.13640 source file (2024-04-21)



LQ

BasicVSR++ with GAN

HifaceGAN

GFPGAN

VQFR

CodeFormer

Ours

GT



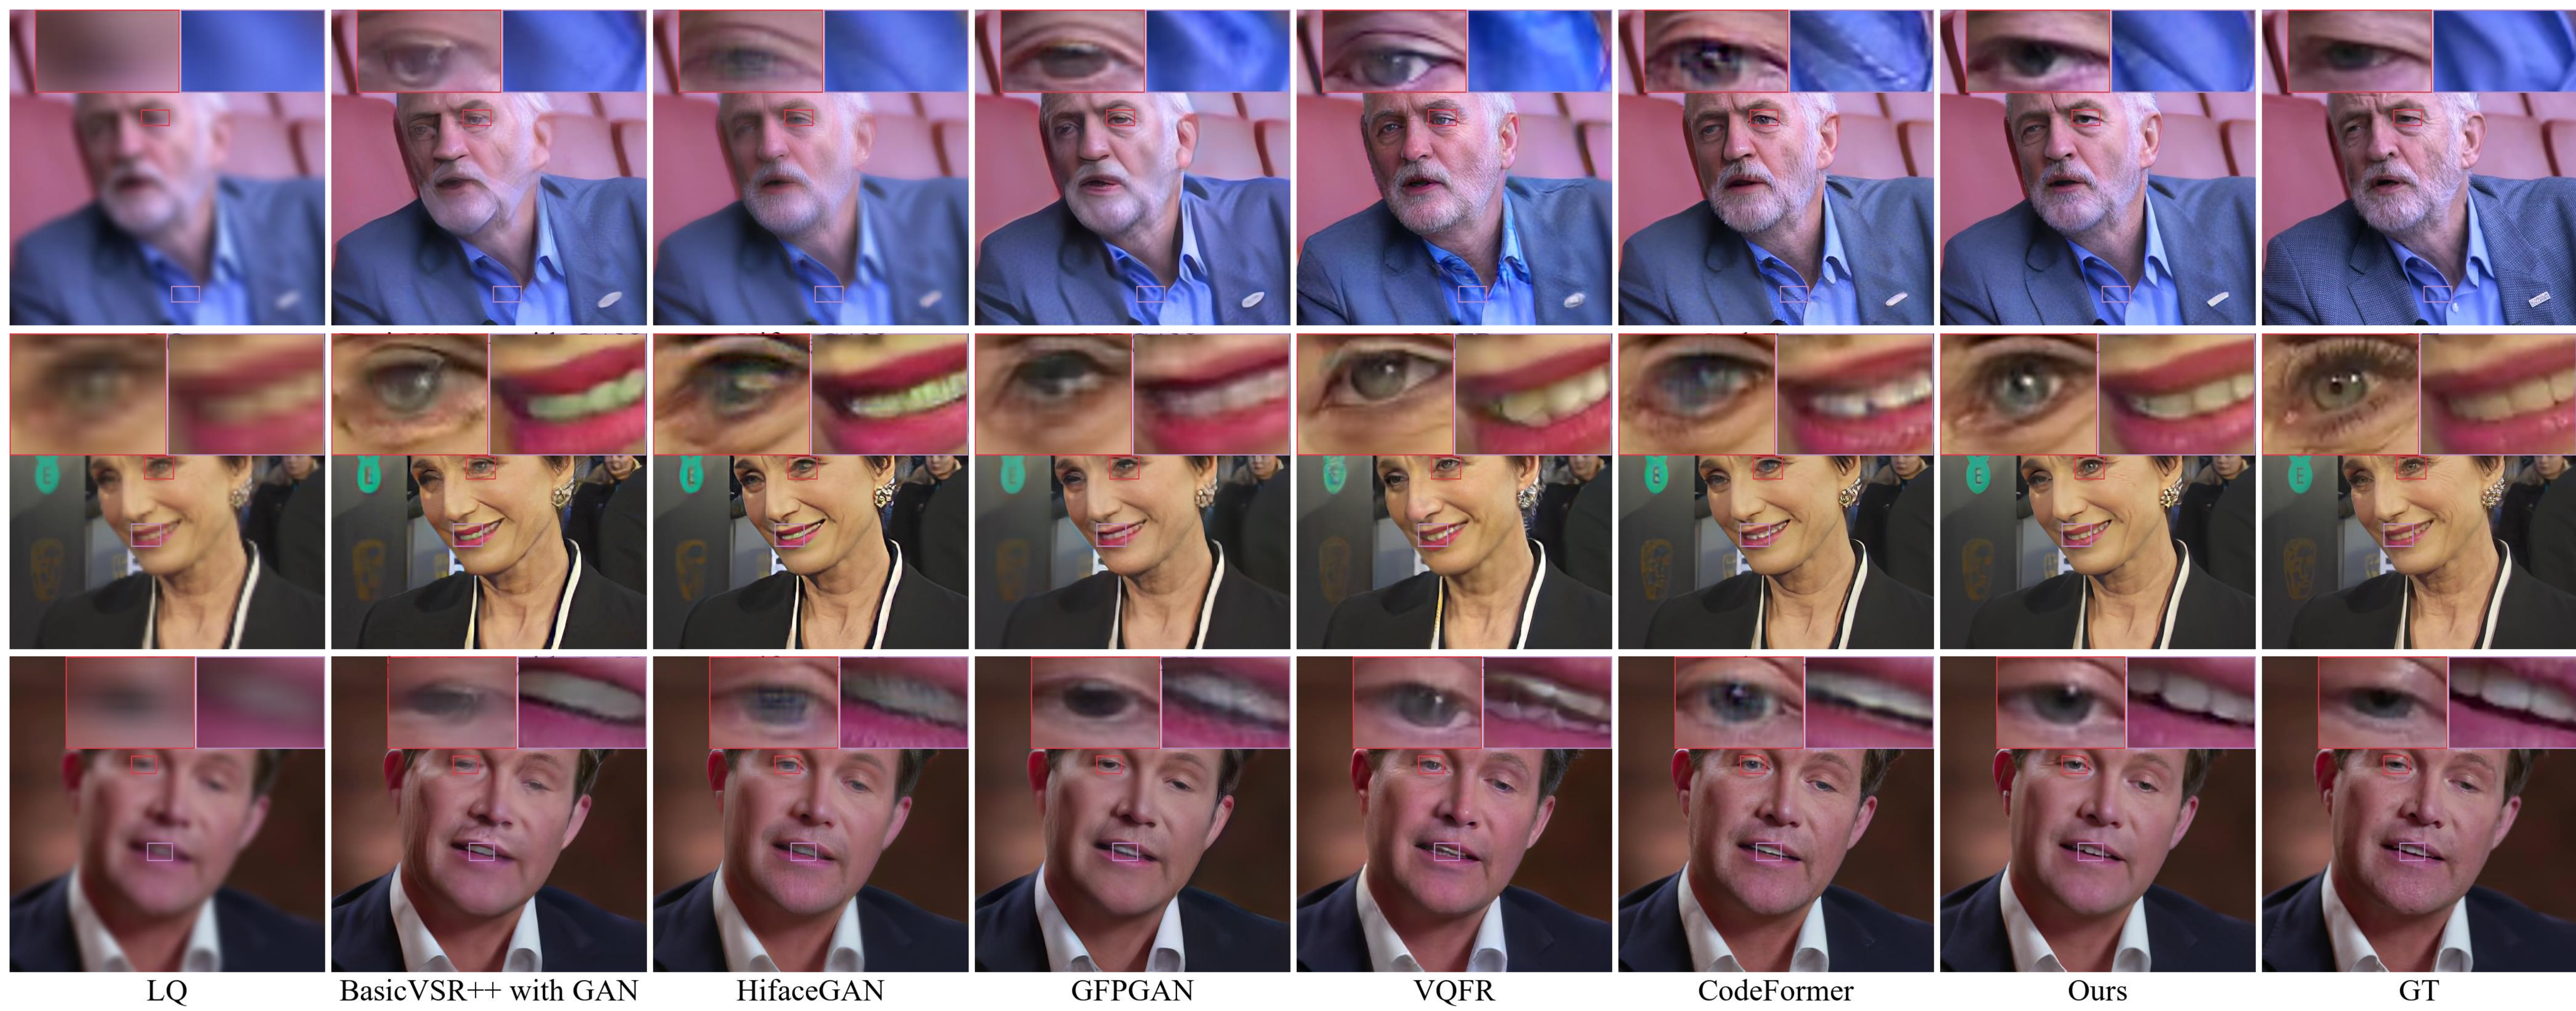

LQ

BasicVSR++ with GAN

HifaceGAN

GFPGAN

VQFR

CodeFormer

Ours

GT





Supplement: Supplementary file 1 [file resultsappendix.pdf]
